# Supplementary material for: Unpaired Weyl nodes from Long-Ranged Interactions: Fate of Quantum Anomalies
Source: arXiv:1804.05078 ancillary file (2018-12-10)
Supplement: Supplementary file 1 [file SingleWeyl_supplement.pdf]

# Supplemental Material: "Single Weyl-Nodes from Long-Ranged Interactions: Fate of Quantum Anomalies"

Tobias Meng and Jan Carl Budich
*Institute of Theoretical Physics, Technische Universität Dresden, 01062 Dresden, Germany*
(Dated: December 10, 2018)

In this supplemental material, we provide further details of the analytical form of the Green's function in the interacting system, and additional plots of density of states.

## I. THE GREEN'S FUNCTION AND ITS LEHMANN REPRESENTATION

The main text is centered around the single-particle density of states, which is proportional to the imaginary part of the fully interacting single-particle retarded Green's function $G^R$. For a translationally invariant system and without magnetic field, $G^R$ has essentially been detailed in Ref. 1 (the main modification of the Hamiltonian in the present work being the momentum-dependence of the interaction), see Eq. (3) in the main text. We are, more generally, also interested in infinite and slab geometries with applied magnetic fields. The magnetic field is implemented in our lattice model via Peierls phases. Because the nodes are separated along $k_z$, we focus on fields along the $z$-direction. This allows us to choose a Landau gauge that adds Peierls factors only for hopping in $x$-direction. The remainder of this section details the calculation of the Green's function for an infinite system. To this end, we first Fourier transform the tight-binding model from $(x, y, z)$ to $\mathbf{k} = (k_x, k_y, k_z)^T$, where $k_x$ is associated with the chosen (magnetic or not magnetic) unit cell. For a given frequency $\omega$ and momentum $\mathbf{k}$, the Green's function $G^R(\omega, \mathbf{k})$ is a $(2N \times 2N)$-matrix, where $N$ is the number of layers in $x$-direction within one (magnetic or not magnetic) unit cell. Without interactions, the Hamiltonian can be diagonalized as $H(\mathbf{k}) = \sum_{\mathbf{k}} \epsilon_{\mathbf{k},n}\, c_{\mathbf{k},m}^\dagger c_{\mathbf{k},m}$ with $m = 1 \dots 2N$ labelling the different eigenlevels. We then construct the $2^{2N}$ many-particle eigenstates by filling up the $2N$ levels with all possible electron numbers, and adding the interaction energy. The latter has a fairly simply form since the interaction Hamiltonian is given by $H_{\text{int}} = \sum_{\mathbf{k}} \frac{U(\mathbf{k})}{2} \left(\sum_m \left(c_{\mathbf{k},m}^\dagger c_{\mathbf{k},m} - 1/2\right)\right)^2$. At fixed momentum $\mathbf{k}$, a many-particle eigenstate $|\alpha, \mathbf{k}\rangle$ with $N_\alpha(\mathbf{k})$ filled levels has the many-particle energy

$$E_\alpha(\mathbf{k}) = \sum_{\text{occupied } m} \epsilon_{\mathbf{k},m} + \frac{U(\mathbf{k})}{2}\left(N_\alpha(\mathbf{k})^2 - 2NN_\alpha(\mathbf{k}) + N^2\right). \tag{S1}$$

The Green's function for electrons in level $m$ is then given by

$$G_m^R(\omega, \mathbf{k}) = \frac{1}{Z}\sum_{\alpha,\beta} \frac{\langle\alpha|c_{\mathbf{k},m}|\beta\rangle\langle\beta|c_{\mathbf{k},m}^\dagger|\alpha\rangle}{\omega + E_\alpha - E_\beta + i\eta}\left(e^{-E_\alpha/k_BT} + e^{-E_\beta/k_BT}\right), \tag{S2}$$

where $T$ denotes the temperature, $\eta \to 0^+$, and $Z$ is the partition sum. We now specialize to zero temperature, in which case either $\alpha$ or $\beta$ needs to be a ground state for the respective term to contribute to $G^R$. Denoting the possibly degenerate ground states of energy $E_{\text{GS}}$ by $|\text{GS}, j\rangle$, where the integer $j$ runs from 1 the number of degenerate ground states, $n_{\text{GS}}$, we have

$$G_m^R(\omega, \mathbf{k}) = \frac{1}{n_{\text{GS}}}\sum_j\sum_\alpha\left(\frac{\langle \text{GS}, j|c_{\mathbf{k},m}^\dagger|\alpha\rangle\langle\alpha|c_{\mathbf{k},m}|\text{GS}, j\rangle}{\omega + E_\alpha - E_{\text{GS}} + i\eta} + \frac{\langle \text{GS}, j|c_{\mathbf{k},m}|\alpha\rangle\langle\alpha|c_{\mathbf{k},m}^\dagger|\text{GS}, j\rangle}{\omega + E_{\text{GS}} - E_\alpha + i\eta}\right). \tag{S3}$$

In this sum, only the terms where $|\alpha\rangle$ differs from $|\text{GS}, j\rangle$ in the level $m$ survive. Denoting the number of particles in the ground state $j$ at momentum $\mathbf{k}$ by $N_{\text{GS},j}(\mathbf{k})$, we use the fact that

$$\frac{U(\mathbf{k})}{2}\left((N_{\text{GS}} \pm 1)^2 - 2N(N_{\text{GS}} \pm 1) + N^2\right) = \frac{U(\mathbf{k})}{2}\left(N_{\text{GS}}^2 - 2NN_{\text{GS}} + N^2\right) + \frac{U(\mathbf{k})}{2}\left(\pm 2(N_{\text{GS}} - N) + 1\right) \tag{S4}$$

to find

$$G_m^R(\omega, \mathbf{k}) = \frac{1}{n_{\text{GS}}}\sum_j\left(\frac{N_{\mathbf{k},m}^j}{\omega - \epsilon_{\mathbf{k},m} - U(\mathbf{k})\left((N_{\text{GS},j}(\mathbf{k}) - N) - \frac{1}{2}\right) + i\eta} + \frac{1 - N_{\mathbf{k},m}^j}{\omega - \epsilon_{\mathbf{k},m} - U(\mathbf{k})\left((N_{\text{GS},j}(\mathbf{k}) - N) + \frac{1}{2}\right) + i\eta}\right), \tag{S5}$$

where $N^j_{\mathbf{k},m} = 0,1$ is the occupancy of the level $m$ in the ground state $j$ for momentum $\mathbf{k}$. To further gain insight into the behavior of the density of states, let us now focus on the case that the ground state is unique for all momenta $\mathbf{k}$. A level that is occupied in the ground state then has the Green's function

$$G^R_{m\ \mathrm{occupied}}(\omega,\mathbf{k}) = \frac{1}{\omega - \epsilon_{\mathbf{k},m} - U(\mathbf{k})\left((N_{\mathrm{GS}}(\mathbf{k}) - N) - \frac{1}{2}\right) + i\eta}, \tag{S6}$$

while the Green's function of an empty level reads

$$G^R_{m\ \mathrm{empty}}(\omega,\mathbf{k}) = \frac{1}{\omega - \epsilon_{\mathbf{k},m} - U(\mathbf{k})\left((N_{\mathrm{GS}}(\mathbf{k}) - N) + \frac{1}{2}\right) + i\eta}. \tag{S7}$$

These expressions elucidate why the density of states shows discontinuities when a single level crosses the chemical potential (as is the case in our simulations in the presence of an applied magnetic field). Since the level is emptied when its energy changes from negative to positive values as a function of $\mathbf{k}$ (with the Fermi level taken to be at zero energy), the number of particles in the ground state $N_{\mathrm{GS}}(\mathbf{k})$ jumps by one. After emptying a level, all other levels are thus shifted to lower energies by an amount of $-U(\mathbf{k})$. The density of states of the level that crosses the chemical potential, however, remains continuous. To understand this last point, consider a level whose energy changes from negative to positive values at momentum $\mathbf{k}_0$ with a positive slope. At the crossing, the number of occupied levels in the ground state changes from $N_0$ to $N_0 - 1$. For smooth interaction functions $U(\mathbf{k})$ (and smooth non-interacting dispersions $\epsilon_{\mathbf{k},m}$), as is the case in our model, we then have

$$\begin{aligned}\lim_{\delta\to 0^+} G^R_m(\omega,\mathbf{k}_0-\delta)\big|_{m\ \mathrm{crossing\ zero}} &= \frac{1}{\omega - \epsilon_{\mathbf{k}_0,m} - U(\mathbf{k}_0)\left((N_0 - N) - \frac{1}{2}\right) + i\eta} \\ &= \frac{1}{\omega - \epsilon_{\mathbf{k}_0,m} - U(\mathbf{k}_0)\left(([N_0-1] - N) + \frac{1}{2}\right) + i\eta} = \lim_{\delta\to 0^+} G^R_m(\omega,\mathbf{k}_0+\delta)\big|_{m\ \mathrm{crossing\ zero}}.\end{aligned} \tag{S8}$$

The density of states of the level crossing zero energy is thus a smooth function of $\mathbf{k}$. We furthermore see that the crossing occurs at the momentum $\mathbf{k}_0$ at which $\epsilon_{\mathbf{k}_0,m} = -U(\mathbf{k}_0)\left((N_0 - N) - \frac{1}{2}\right)$, and is hence shifted to a different momentum as compared to the non-interacting case (in the non-interacting case, the crossing occurs at the momentum $\tilde{\mathbf{k}}_0$ with $\epsilon_{\tilde{\mathbf{k}}_0,m} = 0$).

## II. THE BUMP FUNCTION

In the main text, we employ the bump function

$$b(k,k_0,\delta) = \begin{cases} \exp\left\{-\frac{\delta^2}{(\delta^2-(k-k_0)^2)}\right\} & , \quad k \in [k_0-\delta, k_0+\delta], \\ 0 & , \quad \text{else.} \end{cases} \tag{S9}$$

which we backfold into the first Brillouin zone. As shown in Fig. 1, $b(k,k_0,\delta)$ has a bump-like shape, and it is finite only in a range $2\delta$ around the momentum $k_0$. Its peak value is $b(k_0,k_0,\delta) = e^{-1}$. Note that the bump function is not only smooth, but also differentiable for all degrees of differentiation with respect to $k$.

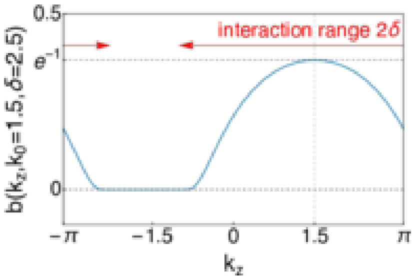


Figure 1: Bump function $b(k_0,k_0,\delta)$ used to smoothly switch on the interaction as a function of momentum $k_z$.

## III. THE DENSITY OF STATES FOR ADDITIONAL MOMENTA

In this section, we provide further plots of the density of states as a function of $k_z$. These plots illustrate that the plots shown in the main text depict the generic behavior when it comes to interaction effects, with the main advantage of cutting through the Weyl nodes (which, in the infinite bulk and at zero magnetic field, are located at $k_x = 0$, $k_y = 0$, and $k_z = \pm k_{\rm Weyl}$). In all plots, and as in the main text, we have chosen $k_{\rm Weyl} = 1.5$ (measuring lengths in units of the unit cell size such that $-\pi \leq k_{x,y,z} < \pi$), $\lambda = 1.5$, while the interaction is chosen as $U(k_z) = U_0\, b(k_z, k_0 = k_{\rm Weyl} = 1.5, \delta = 2.5)$ with $U_0 = 0$ or $U_0 = 2$. To plot the density of states (which really is a sum of Dirac-$\delta$-peaks), we artificially introduce a small spectral broadening in our numerics.

### A. Infinite system at zero magnetic field

First, we show the density of states of an infinite system at vanishing magnetic field. The model can then be solved analytically yielding the single-particle Green's function given in Eq. (S5). To simplify the comparison to plots of the density of states in the presence of a magnetic field, and hence to systems with a magnetic unit cell larger than the atomic unit cell, we here choose to plot the density of states for a unit cell that has been chosen to comprise of 50 layers in $x$-direction (this is hence not the primitive unit cell, and corresponds to backfolding the density of states obtained from Eq. (S5) into the reduced Brillouin zone associated with the enlarged unit cell). The following plots thus complement the plots of the main text, which show the density of states integrated over $k_x$ and $k_y$. In the non-interacting case $U_0 = 0$, the density of states $\rho_{k_x,k_y}(\omega, k_z)$ normalized by its maximal value $\rho_{\rm max}$ is shown in Fig. 2 for $k_x = 0$ (defined in the superlattice, i.e. in the reduced Brillouin zone) and different fixed values of $k_y$, as a function of $\omega$ and $k_z$ (with $k_y = -0.4$, $-0.2$, $-0.1$, $-0.05$, 0, 0.05, 0.1, 0.2, and 0.4 from left to right).

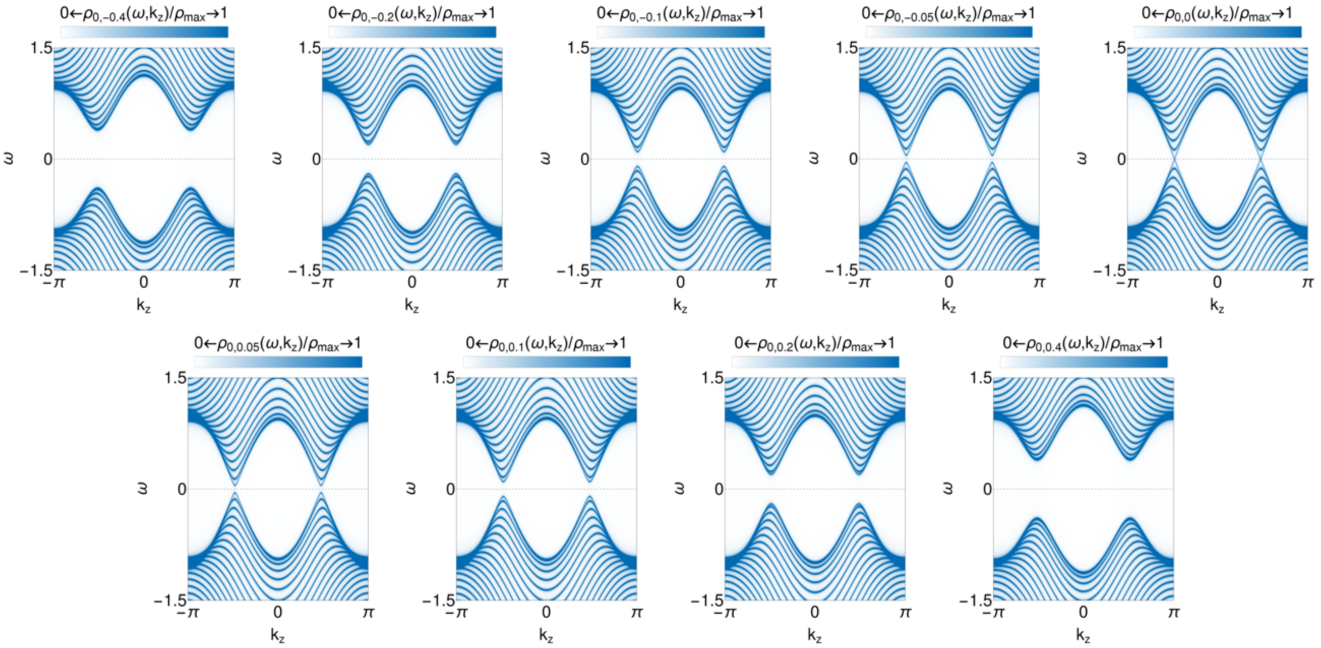


Figure 2: Normalized density of states $\rho_{k_x,k_y}(\omega, k_z)$ for an infinite system with an enlarged unit cell as a function of $\omega$ and $k_z$ at vanishing magnetic field and vanishing interaction strength $U_0 = 0$ for $k_x = 0$ and $k_y = -0.4$, $-0.2$, $-0.1$, $-0.05$, 0, 0.05, 0.1, 0.2, and 0.4 from left to right.

In the interacting case, $U_0 = 2$, we superimpose the non-interacting spectrum shifted by $+U(\mathbf{k})/2$ for states of positive energies and by $-U(\mathbf{k})/2$ for states at negative energies (dashed orange lines). The density of states as $k_y$ is varied is given in Fig. 3.

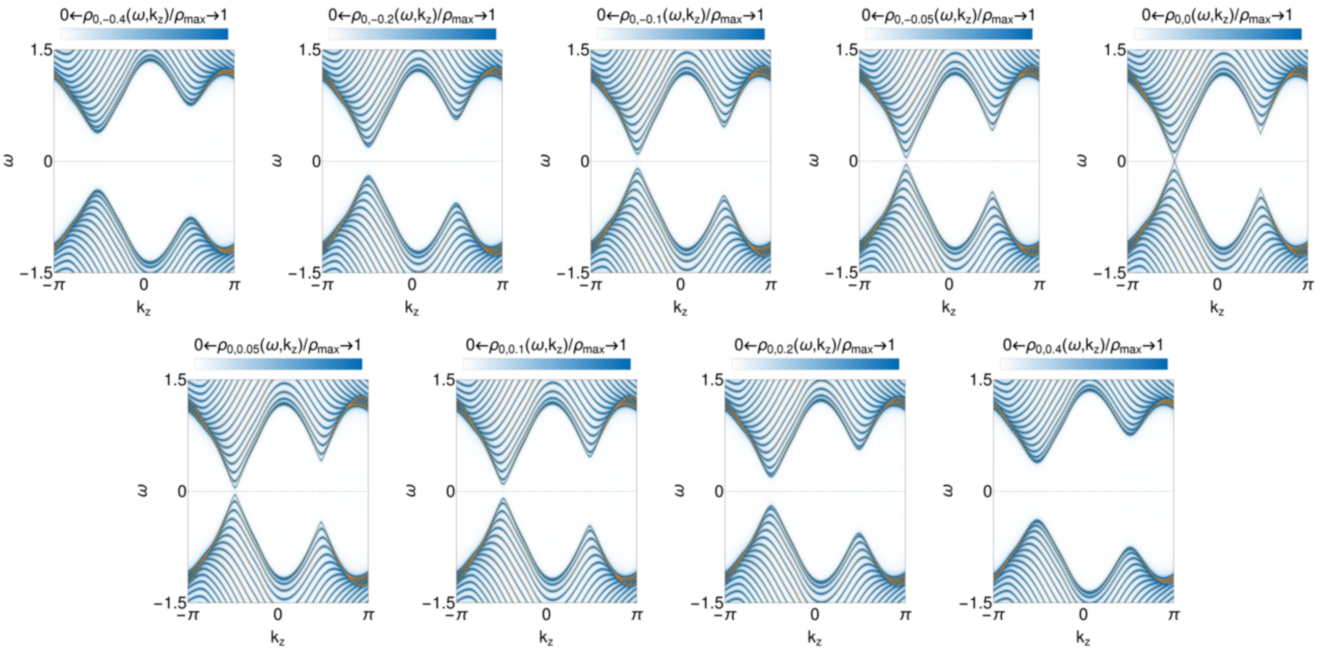


Figure 3: Normalized density of states $\rho_{k_x,k_y}(\omega, k_z)$ for an infinite system with an enlarged unit cell as a function of $\omega$ and $k_z$ at vanishing magnetic field and finite interaction strength $U_0 = 2$ for $k_x = 0$ and $k_y = -0.4$, $-0.2$, $-0.1$, $-0.05$, 0, 0.05, 0.1, 0.2, and 0.4 from left to right.

We thus see that the non-interacting spectrum, shifted by $\pm U(\mathbf{k})/2$, perfectly matches the interacting density of states. This can be understood analytically from Eqs. (S6) and (S7). We furthermore clearly see the gap around the Weyl node at $k_z = +k_{\text{Weyl}} = 1.5$ for all values of $k_y$.

### B. Open boundary conditions at zero magnetic field

Next, we show the density of states $\rho_{k_y}(\omega, k_z)$ normalized by its maximal value $\rho_{\max}$ for a slab of 25 layers in $x$-direction, zero magnetic field, but with open boundary conditions. The reduced number of layers is here chosen such that the level spacing still allows to easily distinguish individual levels (we have checked that the physics is qualitatively unchanged by the reduction from 50 to 25 layers). The open boundary conditions allow us to study the fate of the surface states in the interacting case. In the non-interacting case $U_0 = 0$, the spectral function for different fixed values of $k_y$ as a function of $\omega$ and $k_z$ looks as detailed in Fig. 4 (again for the same values of $k_y$ as before).

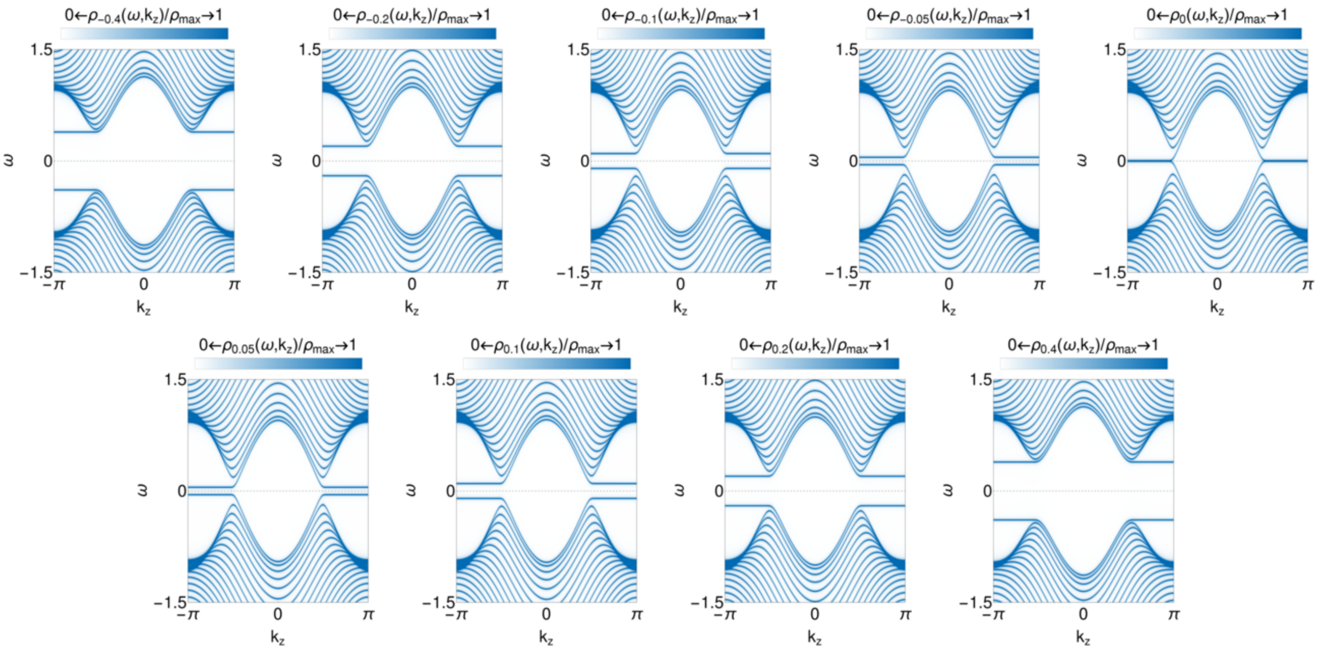


Figure 4: Normalized density of states $\rho_{k_y}(\omega, k_z)$ for a finite slab along $x$ with open boundary conditions as a function of $\omega$ and $k_z$ with open boundary conditions at vanishing magnetic field and vanishing interaction strength $U_0 = 0$ for $k_y = -0.4$, $-0.2$, $-0.1$, $-0.05$, 0, 0.05, 0.1, 0.2, and 0.4 from left to right.

As compared to the case of an infinite system, the main modification is the appearance of surface states that connect with the bulk Weyl nodes (in our simple model Hamiltonian, the surface states are flat as a function of $k_z$ but disperse with $k_y$). The Fermi line of these surface states is a straight line at $k_y = 0$ that merges into to bulk continuum of states at the Weyl nodes. With interactions, and again superimposing the non-interacting spectrum shifted by $\pm U(\mathbf{k})/2$ with dashed orange lines, we find the density of states shown in Fig. 5.

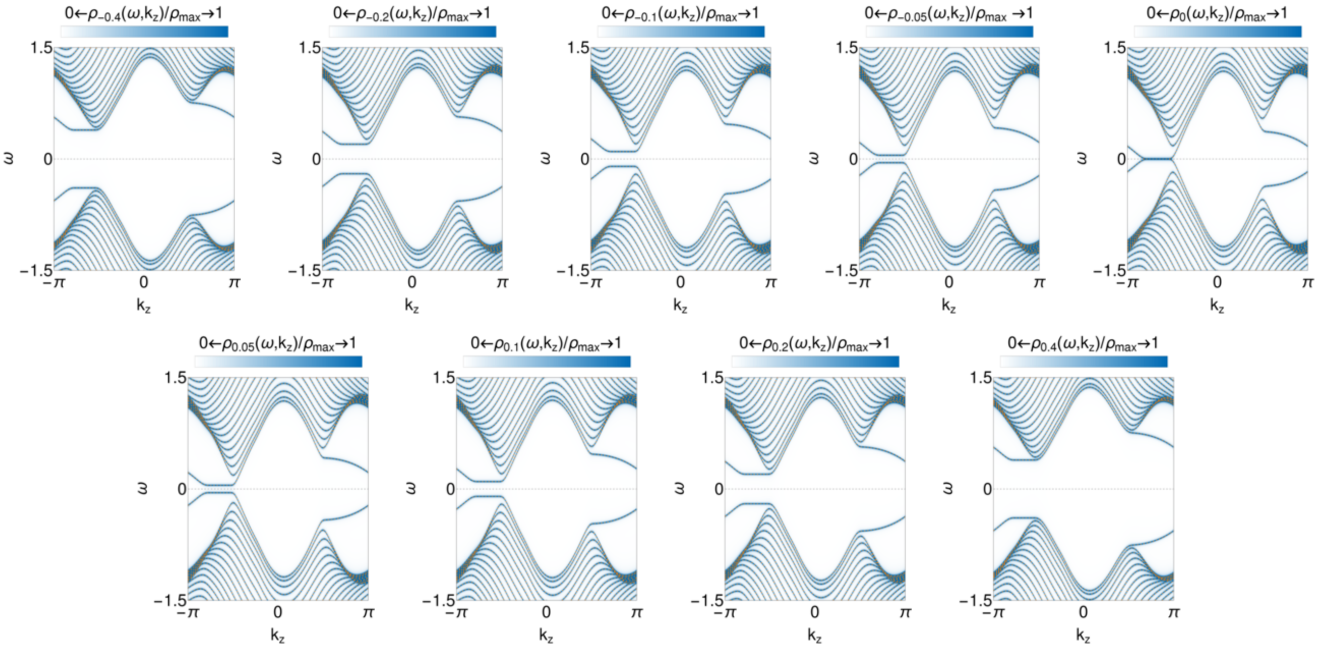


Figure 5: Normalized density of states $\rho_{k_y}(\omega, k_z)$ for a finite slab along $x$ with open boundary conditions at vanishing magnetic field and finite interaction strength $U_0 = 2$ for $k_y = -0.4$, $-0.2$, $-0.1$, $-0.05$, 0, 0.05, 0.1, 0.2, and 0.4 from left to right.

As before, we see that the interaction shifts all energy levels by $\pm U(\mathbf{k})/2$. This in particular also applies to the surface states. The latter thus still smoothly merge with the bulk continuum of states at the Weyl nodes, as is discussed in Ref. 1 using a low-energy approximation. In stark contrast to the prediction of Ref. 1, however, we find that the Fermi line of the surface states (the Fermi-arc) is gapped in the momentum range with finite interaction. This can be understood as a consequence of the non-locality of the interaction $U(\mathbf{k})$ - such an interaction can of course couple, and thus gap out, surface modes on different surfaces.

### C. Infinite system at finite magnetic field along $z$

Next, we add a magnetic field, which we implement via Peierls phases (we neglect the Zeeman effect that – for small enough values of the field – merely shifts the Weyl nodes in momentum space). In a semiclassical picture, the Lorentz force quenches the motion of the electrons in the plane perpendicular to the field by forcing them into cyclotron orbits. The motion parallel to the field, however, remains unaffected. Quantum mechanically, the Weyl node splits up into Landau levels that only disperse parallel to the field. More concretely, the Landau levels of a Weyl Hamiltonian $\hat{H}^{\pm}_{\text{Weyl}} = \pm v_F\, \hat{\sigma} \cdot \hat{\mathbf{q}}$ have energies

$$E_n^{\pm}(k_z) = \begin{cases} \text{sign}(n) v_F \sqrt{k_z^2 + 2eBn} & , \quad n \in \mathbb{Z} \setminus \{0\}, \\ \pm v_F k_z & , \quad n = 0. \end{cases} \tag{S10}$$

The fact that the bulk Landau levels do not disperse perpendicular to the magnetic field remains true in our lattice model to an almost perfect approximation. Let us first turn to the spectral function for an infinite system with a magnetic unit cell of 100 layers in $x$-direction, $B_z = 2\pi/100$, in the absence of interactions, $U_0 = 0$. In agreement with the above discussion of the continuum low-energy model of a Weyl node, we find that the low-energy density of states is almost entirely independent of $k_x$ and $k_y$: only a few levels at high energies (roughly at an energy of half the bandwidth) show a weak dependence of the transversal momenta (not shown). In Fig. 6 below, we show the density of states at $k_x = 0$, $k_y = 0$ as a function of $\omega$ and $k_z$ to illustrate how the density of states $\rho_{k_x,k_y}(\omega, k_z)$ (again normalized by its maximal value $\rho_{\text{max}}$) depends on $k_z$ (left-most plot), while the other plots show the density of states $\rho_{k_x,k_z}(\omega, k_z)$ as a function of $\omega$ and $k_y$ at fixed $k_x = 0$ and $k_z = -0.75$, at fixed $k_x = 0$ and $k_z = 0$, and the normalized $\rho_{k_y,k_z}(\omega, k_z)$ as a function of $\omega$ and $k_x$ at fixed $k_y = 0$ and $k_z = 1.5$ (from left to right). These plots illustrate the quasi-independence of the density of states of $k_x$ and $k_y$.

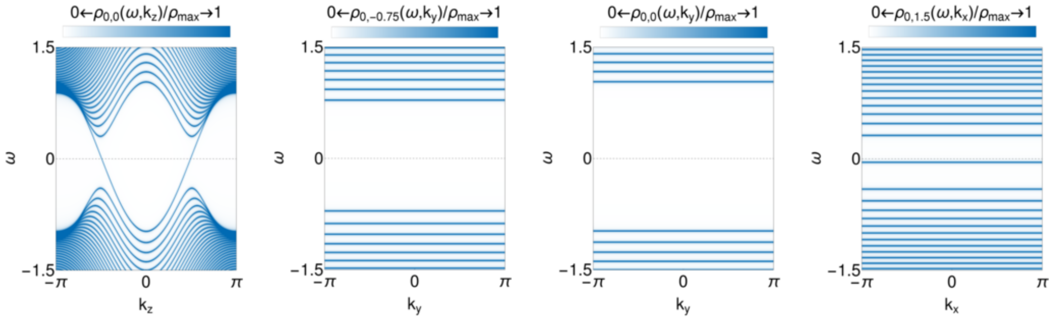


Figure 6: Normalized density of states $\rho_{k_x,k_y}(\omega, k_z)$ for an infinite system at finite magnetic field (using the magnetic unit cell) and vanishing interaction strength $U_0 = 0$ at $k_x = 0$ and $k_y = 0$ as a function of $\omega$ and $k_z$, at $k_x = 0$ and $k_z = -0.75$ and at $k_x = 0$ and $k_z = 0$ as a function of $\omega$ and $k_y$, and at $k_y = 0$ and $k_z = 1.5$ as a function of $\omega$ and $k_x$ (from left to right).

With interactions, $U_0 = 2$, the independence of the density of states of transversal momenta remains true. In Fig. 7, we show the density of states at $k_x = 0$, $k_y = 0$ to illustrate how the density of states depends on $\omega$ and $k_z$ (left-most plot), while the other plots depict the density of states as a function of $\omega$ and $k_y$ at fixed $k_x = 0$ and $k_z = -0.75$, at fixed $k_x = 0$ and $k_z = 0$, and as a function of $\omega$ and $k_x$ at fixed $k_y = 0$ and $k_z = 1.5$ (from left to right).

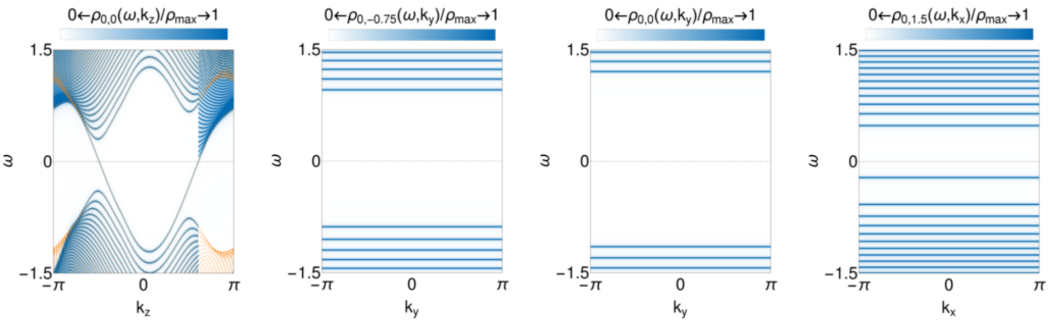


Figure 7: Normalized density of states $\rho_{k_x,k_y}(\omega, k_z)$ for an infinite system at finite magnetic field (using the magnetic unit cell) and finite interaction strength $U_0 = 2$ at $k_x = 0$ and $k_y = 0$ as a function of $\omega$ and $k_z$, at $k_x = 0$ and $k_z = -0.75$ and at $k_x = 0$ and $k_z = 0$ as a function of $\omega$ and $k_y$, and at $k_y = 0$ and $k_z = 1.5$ as a function of $\omega$ and $k_x$ (from left to right).

The dashed orange lines again show the non-interacting spectrum shifted by $\pm U(\mathbf{k})/2$ (the shift is $+U(\mathbf{k})/2$ for the 50 bands with highest energies, and $-U(\mathbf{k})/2$ for the 50 bands with lowest energies), which matches the density of states in the momentum range in which the zeroth Landau level is below zero energy. As discussed in section I, the energies of all levels except the zeroth Landau level show a jump of $-U(\mathbf{k})$ when the zeroth Landau level crosses zero.

### D. Open boundary conditions at finite magnetic field along $z$

We finally discuss spectra of a slab with 100 layers in $x$-direction, a magnetic field of $B_z = 2\pi/100$, and open boundary conditions. In agreement with our above discussions, we find that the bulk levels are almost constant as a function of $k_y$, while the surface states shift with $k_y$. At zero interaction, $U_0 = 0$, this is illustrated by Fig. 8 showing the density of states $\rho_{k_y}(\omega, k_z)$ at fixed $k_y = -0.4$, $-0.2$, $-0.1$, $-0.05$, 0, 0.05, 0.1, 0.2, and 0.4 (from left to right) as a function of $\omega$ and $k_z$.

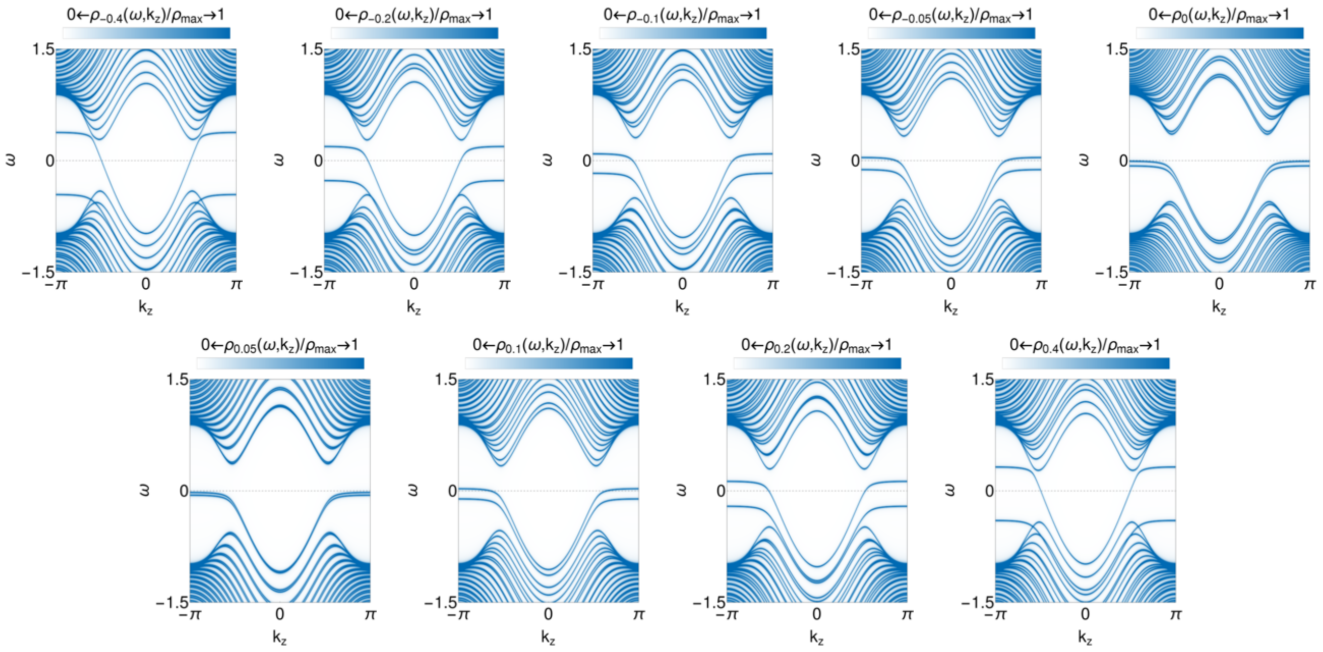


Figure 8: Normalized density of states $\rho_{k_y}(\omega, k_z)$ for a finite slab along $x$ with open boundary conditions at finite magnetic field (using the magnetic unit cell) and vanishing interaction strength $U_0 = 0$ as a function of $\omega$ and $k_z$ for $k_y = -0.4$, $-0.2$, $-0.1$, $-0.05$, 0, 0.05, 0.1, 0.2, and 0.4 from left to right.

With interactions, $U_0 = 2$, we find that the surface states are gapped in the range with strong enough interactions.

In addition, we find that for every left-moving mode crossing the chemical potential, there also is a right-moving partner mode (as discussed in the main text, this is required to ensure global electron number conservation), as shown in Fig. 9.

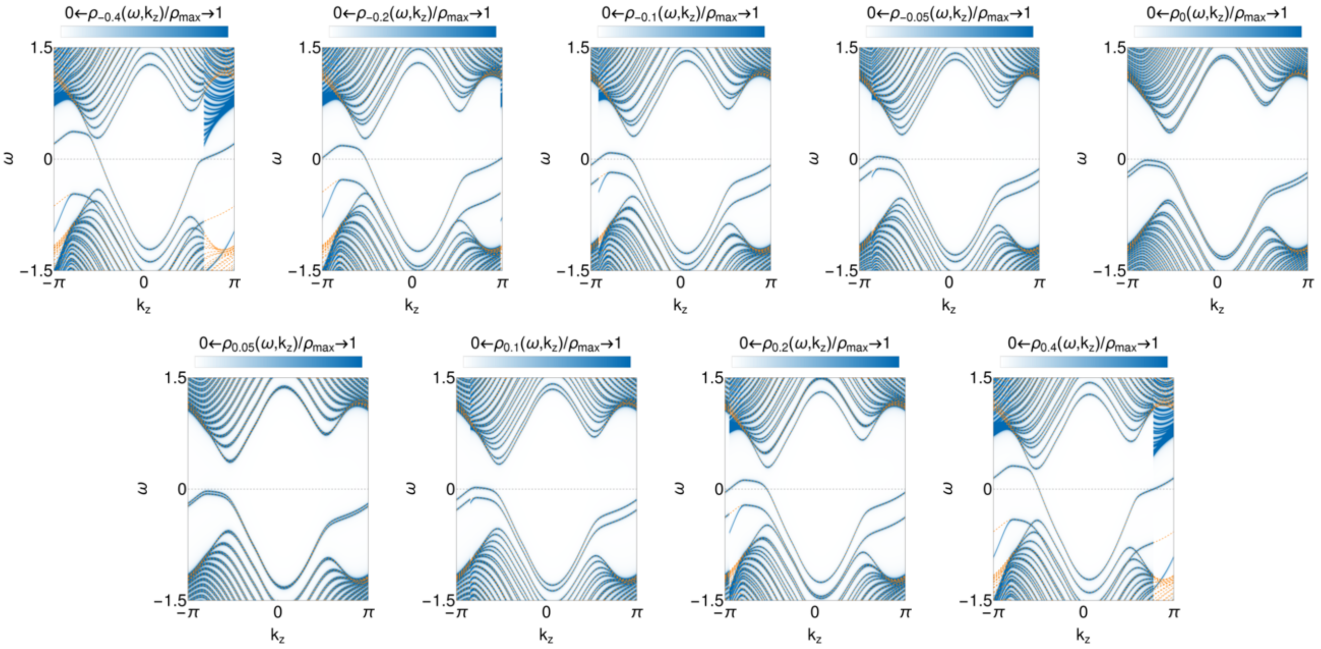


Figure 9: Normalized density of states $\rho_{k_y}(\omega, k_z)$ for a finite slab along $x$ with open boundary conditions at finite magnetic field (using the magnetic unit cell) and finite interaction strength $U_0 = 2$ as a function of $\omega$ and $k_z$ for $k_y = -0.4$, $-0.2$, $-0.1$, $-0.05$, 0, 0.05, 0.1, 0.2, and 0.4 from left to right.

These last plots again depict the density of states at fixed $k_y = -0.4$, $-0.2$, $-0.1$, $-0.05$, 0, 0.05, 0.1, 0.2, and 0.4 (from left to right) as a function of $k_z$, with the non-interacting spectrum shifted by $\pm U(\mathbf{k})$ superimposed for comparison (the shift is $+U(\mathbf{k})/2$ for the 50 bands with highest energies, and $-U(\mathbf{k})/2$ for the 50 bands with lowest energies). As in the case of periodic boundary conditions, levels jump when the surface state/zeroth Landau level-hybrid mode crosses zero.

## IV. FERMI SURFACE EVOLUTION OF A SLAB AS A FUNCTION OF INTERACTION STRENGTH

To provide further insight into the evolution of the Fermi surface as a function of the interaction strength, we also show plots of the density of states $\rho_\omega(k_y, k_z)$ normalized by its maximal value $\rho_{\max}$ for different slabs that are finite along the $x$-direction (and further detailed in the respective subsections). In all cases, we include a finite chemical potential $\mu = 0.1$ to obtain Fermi surfaces that enclose a finite area in the reference setup of a bulk without applied magnetic field (for $\mu = 0$, the Fermi surface would be just two points: the Weyl nodes). Overall, we see that interactions shift the individual levels by $\pm U(\mathbf{k})/2$ as above, that whenever a level crosses the Fermi surface, the other levels jump, and finally that the numbers of right- and left-moving modes crossing the chemical potential are equal. In all cases show below, we show the density of states at $k_y = 0$ as a function of $\omega$ and $k_z$ for reference in the upper row, and plot the Fermi surfaces (the density of states at $\omega = 0$ as a function of $k_y$ and $k_z$) in the lower row.

### A. Periodic boundary conditions at zero magnetic field

We begin with the most simple case: a slab with periodic boundary conditions in the absence of a magnetic field (for a slab with 50 layers in $x$-direction), and with interaction strengths $U_0 = 0$, $U_0 = 0.25$, $U_0 = 0.5$, and $U_0 = 0.75$ (from left to right). The density of states and Fermi surfaces are shown in Fig. {ref:fig:fs

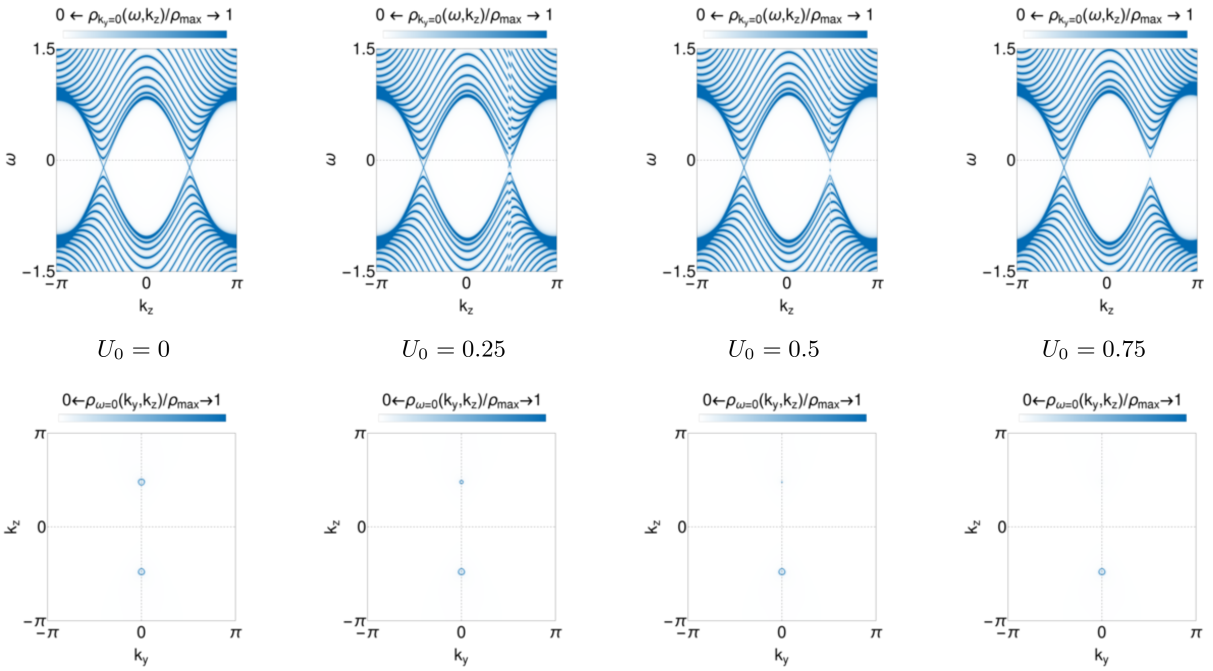


Figure 10: Top row: normalized density of states $\rho_{k_y}(\omega, k_z)$ for a finite slab along $x$ with periodic boundary conditions at vanishing magnetic field as a function of $\omega$ and $k_z$ for $k_y = 0$ with varying interaction strength $U_0 = 0$, $U_0 = 0.25$, $U_0 = 0.5$, and $U_0 = 0.75$ from left to right. Bottom row: associated Fermi surfaces, i. e. the normalized density of states $\rho_{k_y}(\omega, k_z)$ at fixed $\omega = 0$ as a function of $k_y$ and $k_z$, again for $U_0 = 0$, $U_0 = 0.25$, $U_0 = 0.5$, and $U_0 = 0.75$ from left to right.

We find that the Fermi surface shrinks continuously as the interaction strength is reduced until the Fermi surface associated with the gapped node is gone.

## B. Open boundary conditions at zero magnetic field

Next, we plot the density of states of a slab with open boundary conditions in the absence of a magnetic field for a slab with 25 layers in $x$-direction, and with interaction strengths $U_0 = 0$, $U_0 = 0.5$, $U_0 = 1$, and $U_0 = 2$ (from left to right) in Fig. 11.

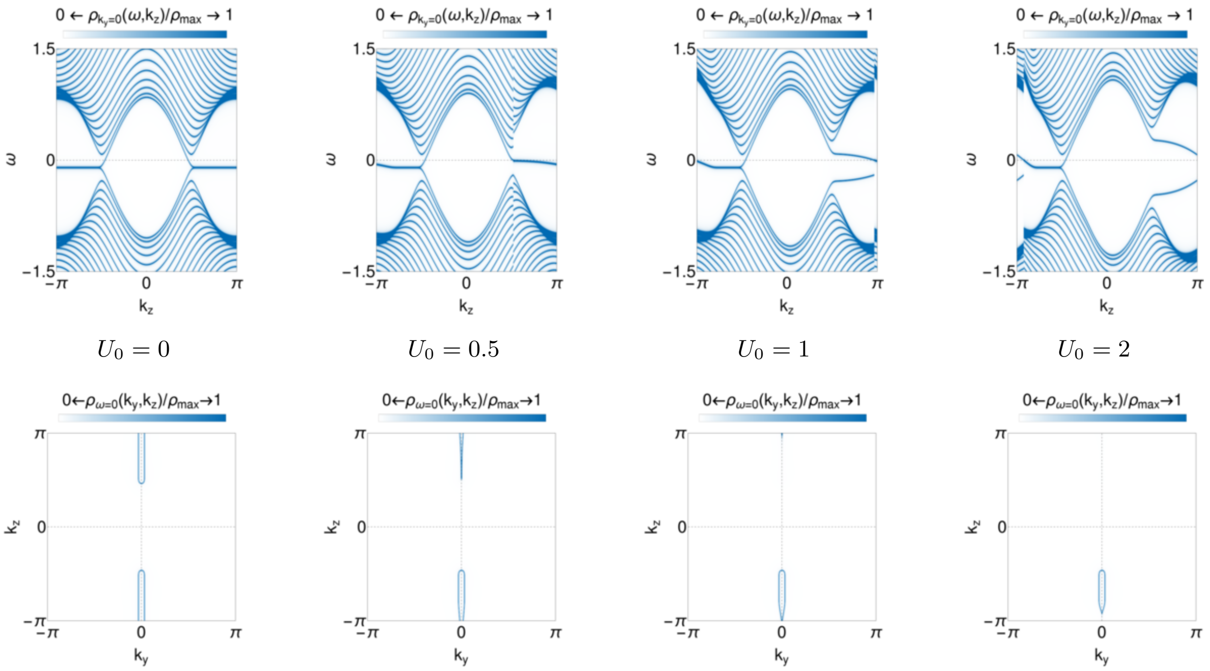


Figure 11: Top row: normalized density of states $\rho_{k_y}(\omega, k_z)$ for a finite slab along $x$ with open boundary conditions at vanishing magnetic field as a function of $\omega$ and $k_z$ for $k_y = 0$ with varying interaction strength $U_0 = 0$, $U_0 = 0.5$, $U_0 = 1$, and $U_0 = 2$ from left to right. Bottom row: associated Fermi surfaces, i. e. the normalized density of states $\rho_{k_y}(\omega, k_z)$ at fixed $\omega = 0$ as a function of $k_y$ and $k_z$, again for $U_0 = 0$, $U_0 = 0.5$, $U_0 = 1$, and $U_0 = 2$ from left to right.

As compared to the case of periodic boundary conditions, the main new feature in Fig. 11 is the appearance of the surface states at the Fermi level. The Fermi surface, including the surface states, again smoothly shrinks as the interaction strength is increased.

### C. Periodic boundary conditions at finite magnetic field along $z$

In Fig. 12, we show the evolution of the density of states of a slab with periodic boundary conditions with 100 layers in $x$-direction in a finite magnetic field along $z$ (with the smallest possible field commensurate with the slab, $B_z = 2\pi/100$, and with $U_0 = 0$, $U_0 = 0.5$, $U_0 = 1$, and $U_0 = 2$ from left to right).

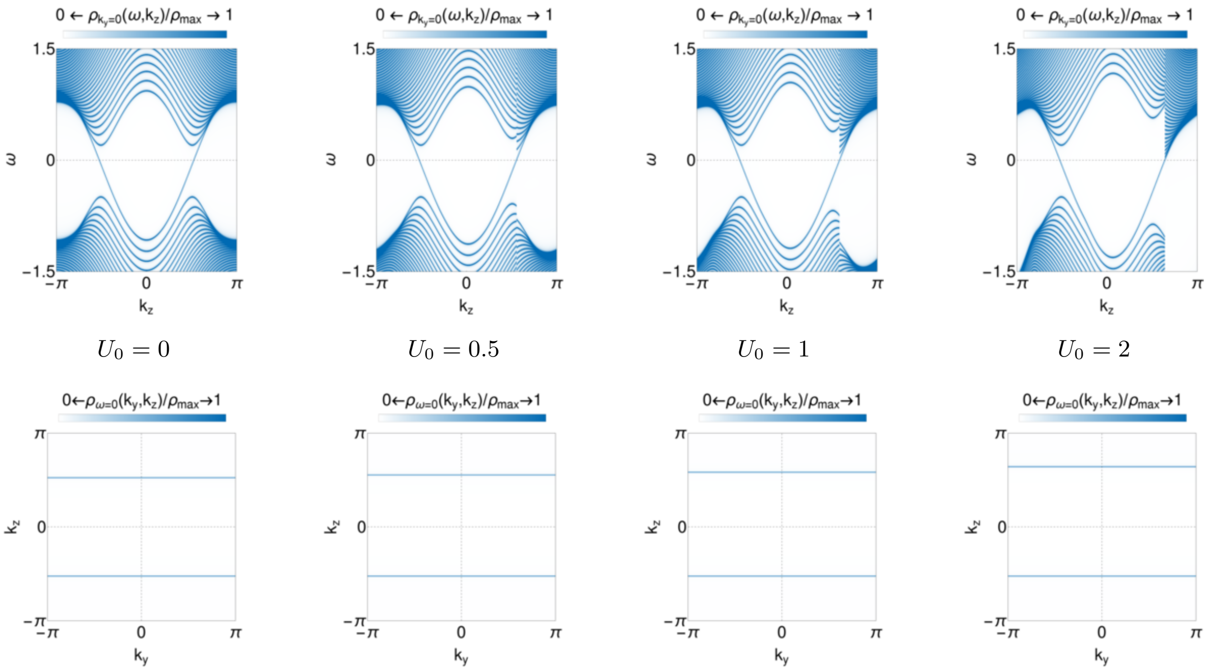


Figure 12: Top row: normalized density of states $\rho_{k_y}(\omega, k_z)$ for a finite slab along $x$ with periodic boundary conditions at finite magnetic field as a function of $\omega$ and $k_z$ for $k_y = 0$ with varying interaction strength $U_0 = 0$, $U_0 = 0.5$, $U_0 = 1$, and $U_0 = 2$ from left to right. Bottom row: associated Fermi surfaces, i. e. the normalized density of states $\rho_{k_y}(\omega, k_z)$ at fixed $\omega = 0$ as a function of $k_y$ and $k_z$, again for $U_0 = 0$, $U_0 = 0.5$, $U_0 = 1$, and $U_0 = 2$ from left to right.

We find that the interaction shifts the Fermi-level-crossing of the chiral Landau level with positive velocity to larger momenta $k_z$, which is a direct consequence of the shift the chiral Landau level by an energy of $\Delta E = -U(\mathbf{k})/2$ discussed in Sec. III C and the main text.

### D. Open boundary conditions at finite magnetic field along $z$

In Fig. 13, finally, we depict the evolution of the density of states of a slab with open boundary conditions with 100 layers in $x$-direction at finite magnetic field along the $z$-direction (with the smallest possible field commensurate with the slab, $B_z = 2\pi/100$, and for $U_0 = 0$, $U_0 = 0.5$, $U_0 = 1$, $U_0 = 2$ from left to right).

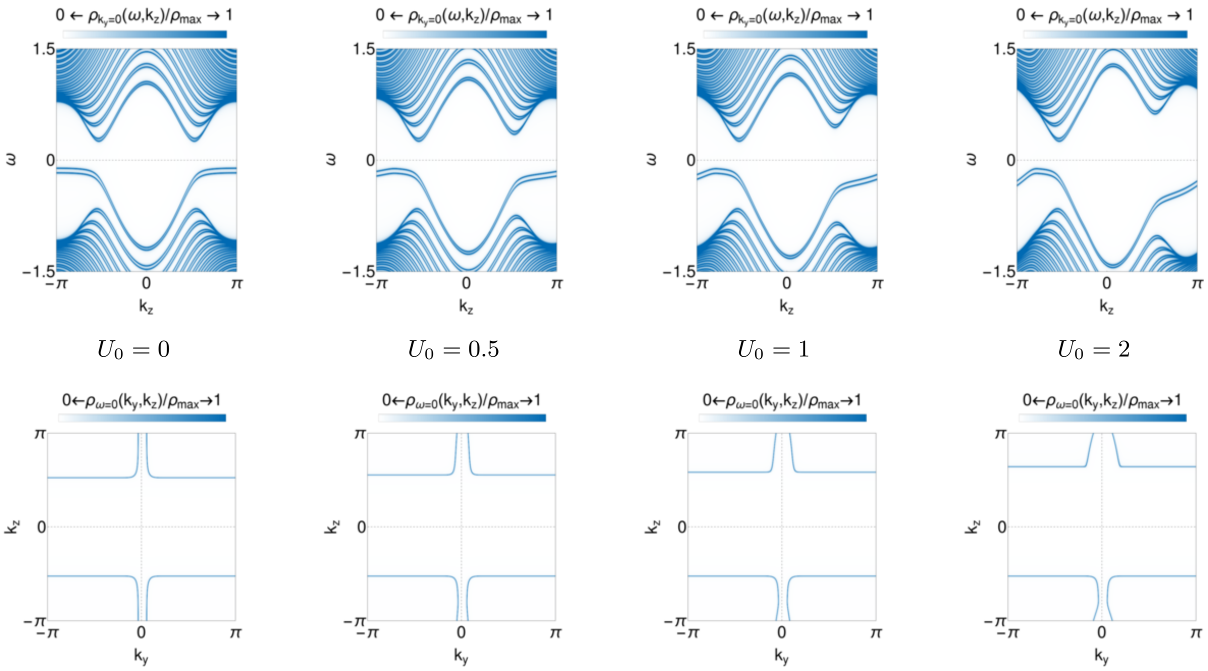


Figure 13: Top row: normalized density of states $\rho_{k_y}(\omega, k_z)$ for a finite slab along $x$ with open boundary conditions at finite magnetic field as a function of $\omega$ and $k_z$ for $k_y = 0$ with varying interaction strength $U_0 = 0$, $U_0 = 0.5$, $U_0 = 1$, and $U_0 = 2$ from left to right. Bottom row: associated Fermi surfaces, i. e. the normalized density of states $\rho_{k_y}(\omega, k_z)$ at fixed $\omega = 0$ as a function of $k_y$ and $k_z$, again for $U_0 = 0$, $U_0 = 0.5$, $U_0 = 1$, and $U_0 = 2$ from left to right.

We see that the interaction not only pushes the bulk Fermi line to larger momenta $k_z$ (as in the last subsection), but also pushes the surface state Fermi line away from $k_y = 0 = 2\pi$. In a magnetic field, the $k_y$-quantum number also indicates the guiding center position. In real space, the surface states at the Fermi level are thus pushed away from the actual surfaces, which may be interpreted as a precursor of the "annihilation" of states at the Fermi level for a given $k_z$ as the interaction strength is increased (this annihilation is driven by the infinitely long-ranged interaction coupling states on opposite surfaces of the slab).

## V. EVOLUTION OF THE DENSITY OF STATES UPON VARYING THE INTERACTING MOMENTUM RANGE $\delta$

In this section, we are interested in how the density of states changes when the interaction is finite over larger or smaller widths $\delta$. The former sections of the Supplemental Material and the main text suggest that the interaction essentially shifts the density of states by $\pm U(\vec{k})/2$, and that crossings of chiral Landau levels cause jumps due to the discontinuous change in the number of occupied states, and hence of the interaction energy. This picture suggests that a variation of the interaction width $\delta$ does not lead to qualitatively new physics as long as one node remains gapless. To test this intuition, we calculate the density of states for three different interaction widths $\delta = 0.5$, $\delta = 1.5$, and $\delta = 2.5$. The results are shown in FIg. 14. In all cases, we use $U_0 = 2$, $k_{\text{Weyl}} = 1.5$ and $\lambda = 1.5$. We simulate:

(i) the density of states $\rho_{k_x,k_y}(\omega, k_z)$ of an infinite system with a unit cell of 50 layers in $x$ direction for $k_x = k_y = 0$ at zero magentic field (normalized to its maximal value $\rho_{\max}$),

(ii) the density of states $\rho_{k_y}(\omega, k_z)$ of a system with open boundary conditions (OBC) in $x$-direction and a width of 25 layers for $k_y = 0$ at zero magentic field (normalized to its maximal value $\rho_{\max}$),

(iii) the density of states $\rho_{k_x,k_y}(\omega, k_z)$ of an infinite system with a unit cell of 100 layers in $x$ direction for $k_x = k_y = 0$ subject to a magnetic field of $B_z = 2\pi/100$ (normalized to its maximal value $\rho_{\max}$),

(iv) the density of states $\rho_{k_y}(\omega, k_z)$ of a system with open boundary conditions in $x$-direction and a width of 100 layers for $k_y = 0$ subject to a magnetic field of $B_z = 2\pi/100$ (normalized to its maximal value $\rho_{\max}$).

In all cases, the vertical dashed red lines indicate the position of the Weyl nodes in the non-interacting system. The density of states depicted below indeed show that increasing the interaction range $\delta$ merely implies that the shift by $\pm U(\vec{k})/2$ extend over a larger portion of momentum space.

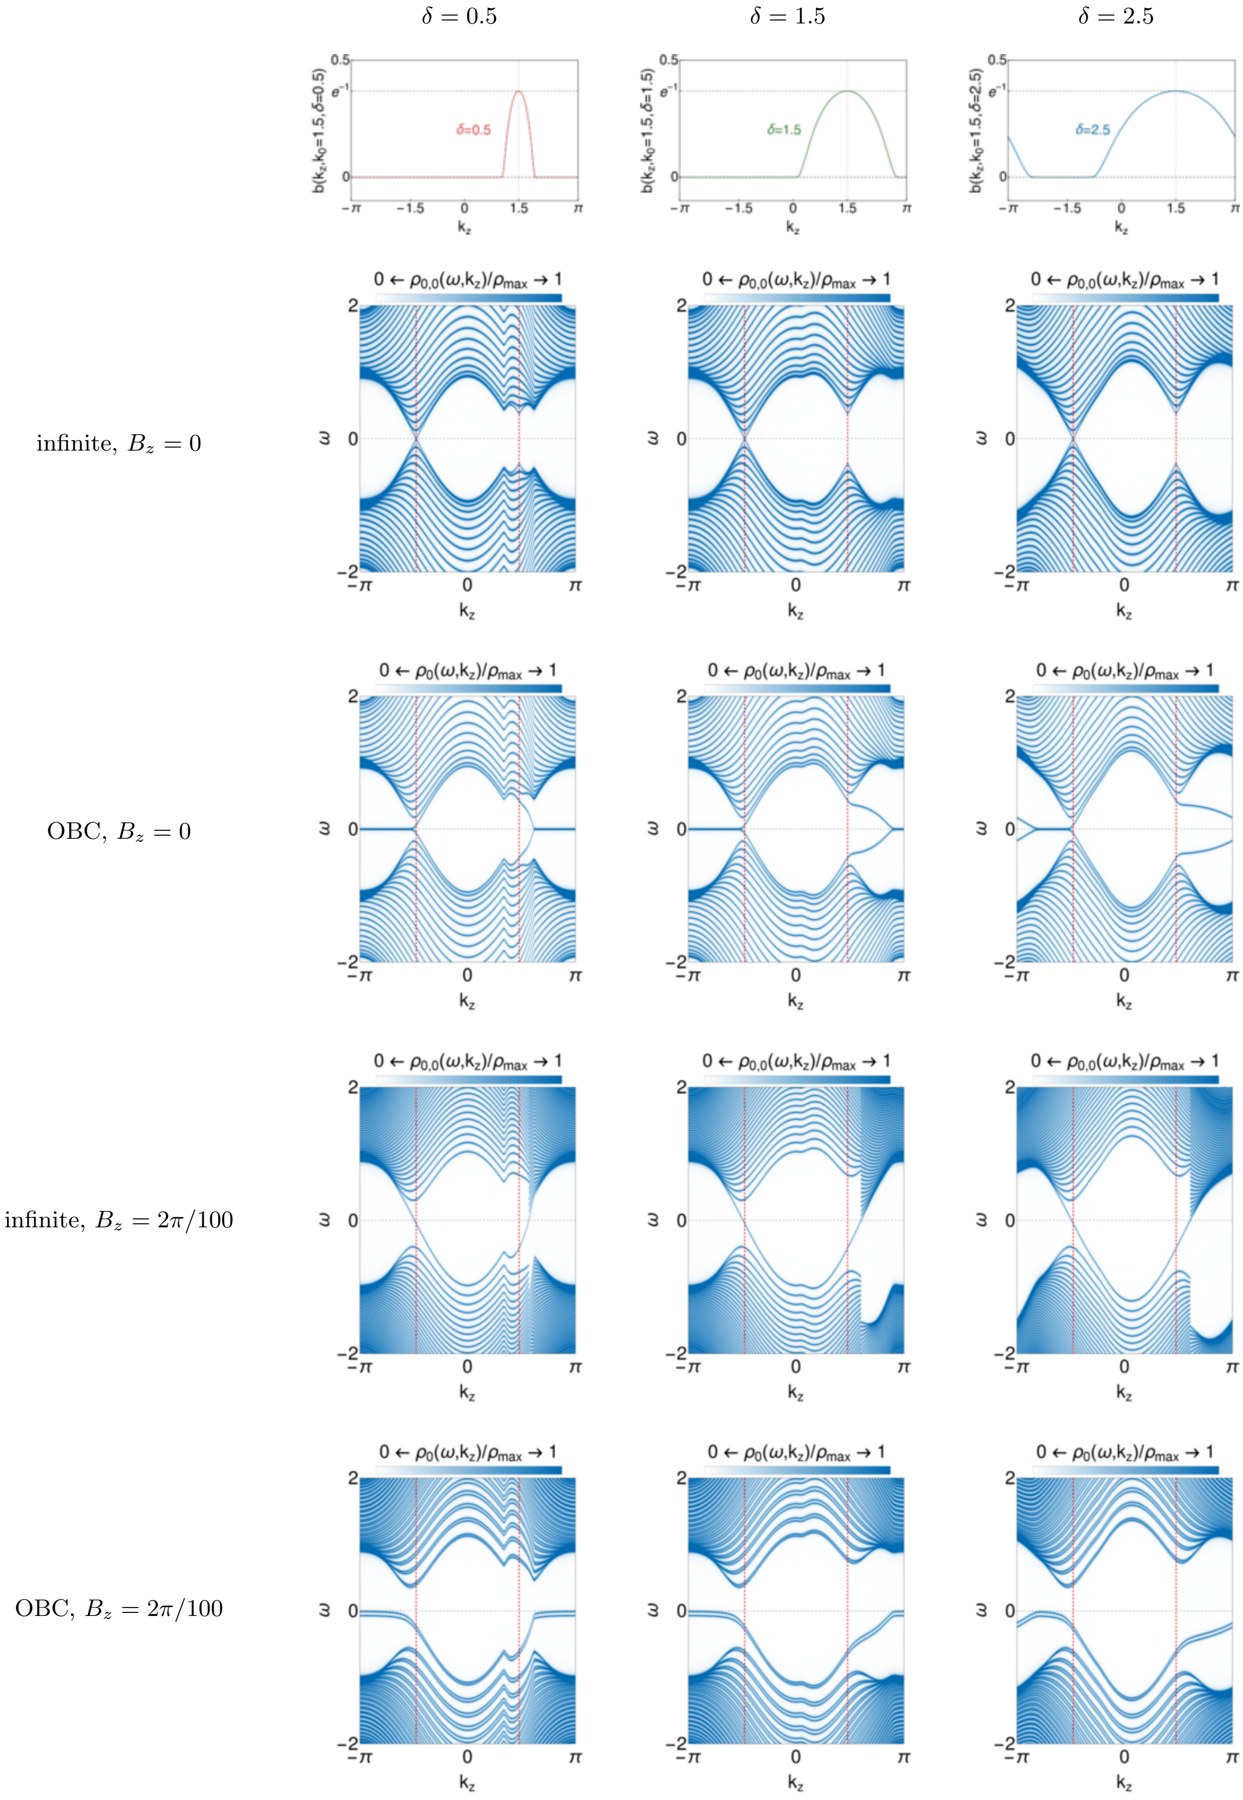


Figure 14: First row: interaction profiles as a function of $k_z$. Second row: normalized density of states $\rho_{k_x,k_y}(\omega, k_z)$ as a function of $\omega$ and $k_z$ for an infinite system at vanishing magnetic field in the enlarged unit cell for the interaction profiles depicted in the first row. Third row: normalized density of states $\rho_{k_y}(\omega, k_z)$ as a function of $\omega$ and $k_z$ for a finite slab with open boundary conditions (OBC) system at vanishing magnetic field for the interaction profiles depicted in the first row. Fourth row: normalized density of states $\rho_{k_x,k_y}(\omega, k_z)$ as a function of $\omega$ and $k_z$ for an infinite system at finite magnetic field (using the magnetic unit cell) for the interaction profiles depicted in the first row. Fifth row: normalized density of states $\rho_{k_y}(\omega, k_z)$ as a function of $\omega$ and $k_z$ for a finite slab with open boundary conditions system at finite magnetic field for the interaction profiles depicted in the first row.

## VI. OTHER INTERACTION PROFILES: DOUBLE PEAK STRUCTURE

Another important question concerns the dependence of the density of states on the qualitative shape of the interaction profile. The case of a constant interaction amplitude, $U(\vec{k}) = U_0 \; \forall \vec{k}$, has been discussed in Ref. 1: such a constant interaction gaps out both Weyl nodes. Here, we turn to another interesting interaction profile, namely a double peak structure with a finite interaction at both Weyl node momenta, but with a range of zero interaction an intermediate momenta. More precisely, we focus on the interaction profile $U(\vec{k}) = U_0 \, b_2(k_z, k_{\text{Weyl}}, \delta = 1.25)$ with $b_2(k_z, k_{\text{Weyl}}, \delta) = b(k_z, k_{\text{Weyl}}, \delta) + b(k_z, -k_{\text{Weyl}}, \delta)$, which for $k_{\text{Weyl}} = 1.5$ and $\delta = 1.25$ looks as shown in Fig. 15.

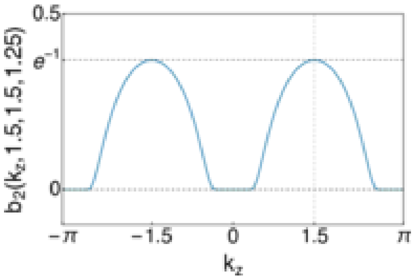


Figure 15: Alternative bump function $b_2(k_0, k_0, \delta)$ used to smoothly switch on the interaction as a function of momentum $k_z$.

We calculate the density of states for a system subject to this interaction profile (using $U_0 = 2$, $k_{\text{Weyl}} = 1.5$ and $\lambda = 1.5$ as before, and setting the width of each interaction peak to be $\delta = 1.25$). In all following plots, the density of states is normalized by its maximal value $\rho_{\text{max}}$, and vertical dashed red lines indicate the position of the Weyl nodes in the non-interacting case. We first show that, as one expects, the double-peak interaction gaps out both Weyl nodes by simulating an infinite system with the unit cell chosen to contain 50 layers in $x$-direction. The density of states $\rho_{k_x=0,k_y=0}(\omega, k_z)$ is given in Fig. 17.

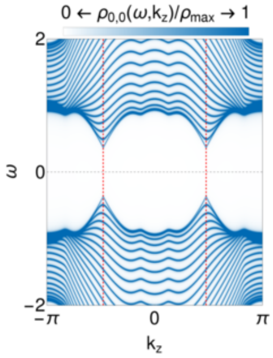


Figure 16: Normalized density of states $\rho_{k_x,k_y}(\omega, k_z)$ for an infinite system with an enlarged unit cell as a function of $\omega$ and $k_z$ at $k_x = 0$ and $k_y = 0$ at vanishing magnetic field and with the alternative interaction profile shown in Fig. 15.

With open boundary conditions along $x$, we find that the density of states $\rho_{k_y=0}(\omega, k_z)$ is gapped for all momenta with a finite interaction. In contrast, the surface states remain gapless in the momentum range that has $U(k_z) = 0$. There are thus residual segments of the Fermi arc that are not connected to gapless Weyl nodes, but instead detach from zero energy for momenta with a finite interaction (this can be understood as a consequence of the long-range nature of the interaction that allows to coupled counter-propagating edge states at opposite surfaces). For a slab with 25 layers in $x$-direction, the density of states is shown in Fig. 17

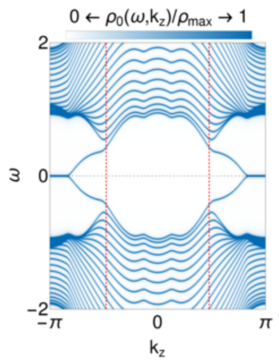


Figure 17: Normalized density of states $\rho_{k_y}(\omega, k_z)$ for a finite slab with open boundary conditions as a function of $\omega$ and $k_z$ at $k_y = 0$ at vanishing magnetic field and with the alternative interaction profile shown in Fig. 15.

Next, we turn to an infinite system with a unit cell of 100 layers in $x$-direction subject to a magnetic field $B_z = 2\pi/100$ (with $k_x = k_y = 0$). We find that the double peak structure of the interaction causes the Landau levels of both Weyl nodes to be shifted. As a result, the zero-energy crossings of both zeroth Landau levels occur at momenta away from the Weyl nodes. Much like in the case of a single gapless node, the chiral anomaly remains untouched, now even despite the complete lack of bulk Weyl nodes at zero magnetic field. Again, this can be understood from the constraint of global electron number conservation: while, without bulk Weyl nodes, the existence of chiral Landau levels at zero energy hinges on the details of the interaction profile (for example on whether it decreases to zero at momenta away from the nodes), we find that *if* chiral Landau levels are present, they *have to* come in counter-propagating pairs. This is indeed shown by the density of states $\rho_{k_x=0,k_y=0}(\omega, k_z)$ in Fig. 18.

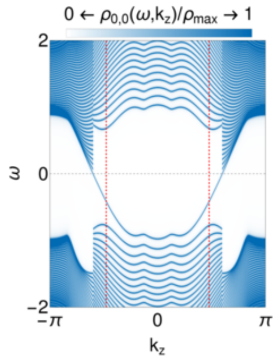


Figure 18: Normalized density of states $\rho_{k_x,k_y}(\omega, k_z)$ for an infinite system slab (using the magnetic unit cell) as a function of $\omega$ and $k_z$ at $k_x = 0$ and $k_y = 0$ at finite magnetic field and with the alternative interaction profile shown in Fig. 15.

Finally, we turn to a system with open boundary conditions, 100 layers in $x$-direction subject to a magnetic field $B_z = 2\pi/100$, and $k_y = 0$. We find that here as well, the chiral Landau level/Fermi arc surface state survives in principle, but is shifted in the momentum range with finite interactions. The density of states $\rho_{k_y=0}(\omega, k_z)$ looks as depicted in Fig. 19.

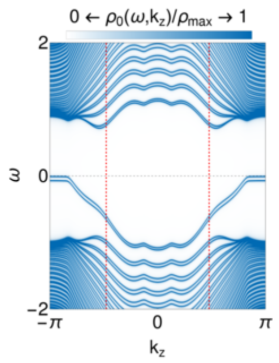


Figure 19: Normalized density of states $\rho_{k_y}(\omega, k_z)$ for a finite slab with open boundary conditions as a function of $\omega$ and $k_z$ at $k_y = 0$ at finite magnetic field and with the alternative interaction profile shown in Fig. 15.

## VII. MULTIORBITAL MODEL WITH NODES IN DIFFERENT ORBITALS

One key ingredient in the discussion of the main text is the fact that the interaction does not couple the two Weyl nodes. One possible physical mechanism providing such a situation is an orbital-selective interaction: if the states associated with one of the Weyl nodes live in orbital $A$, while the states associated with the other node live in orbital $B$, and if the interaction only couples electrons in orbital $B$, then the interaction vanishes at the Weyl node living in orbital $A$.

Here, we show that a system with two orbitals per site (or two atoms in the unit cell) is already sufficient to achieve an orbital distinction of the Weyl nodes. As a minimal model, we use the tight-binding Hamiltonian

$$H = \sum_{\mathbf{k}} \Psi^\dagger_{\mathbf{k}} \, \mathcal{H}_{\mathbf{k}} \, \Psi_{\mathbf{k}} \tag{S11}$$

with the spinor $\Psi^\dagger_{\mathbf{k}} = (c^\dagger_{\mathbf{k},\uparrow,A}, c^\dagger_{\mathbf{k},\downarrow,A}, c^\dagger_{\mathbf{k},\uparrow,B}, c^\dagger_{\mathbf{k},\downarrow,B})$ containing the creation operators $c_{\mathbf{k},\sigma,i}$ for electrons of spin $\sigma =\uparrow,\downarrow$ in orbital $A, B$, and where

$$\mathcal{H}_{\mathbf{k}} = h_{\mathbf{k}} \, \frac{\mathbb{1}_\tau + (\cos(k_z) - \cos(k_{\mathrm{Weyl}}))\, \tau_x + \sin(k_z)\, \tau_z}{2} + (h_{\mathbf{k}} + \delta E \, \mathbb{1}_\sigma)\, \frac{\mathbb{1}_\tau - (\cos(k_z) - \cos(k_{\mathrm{Weyl}}))\, \tau_x - \sin(k_z)\, \tau_z}{2}, \tag{S12}$$

$$h_{\mathbf{k}} = \sin(k_x)\, \sigma_x + \sin(k_y)\, \sigma_y + (\cos(k_z) - \cos(k_{\mathrm{Weyl}}) + \lambda\, (2 - \cos(k_x) - \cos(k_y)))\, \sigma_z - \mu \, \mathbb{1}_\sigma, \tag{S13}$$

where $\sigma_i$ are Pauli matrices acting on the spin degree of freedom, while $\tau_i$ are Pauli matrices acting on the orbital pseudo-spin (orbital $A$ corresponds to the $\tau_z$-eigenstate with eigenvalue $-1$, while orbital $B$ corresponds to the $\tau_z$-eigenvalue $+1$). In the following, we set $k_{\mathrm{Weyl}} = \pi/2$, $\lambda = 1.5$, and $\mu = 0$. The parameter $\delta E$ is an energy shift for the two additional bands that we shift away from the chemical potential by setting $\delta E = 10$.

Upon diagonalization, we find that this model features two pairs of bands split by $\delta E$. Each pair of bands features two Weyl nodes that live in different orbitals, as indicated by the following spectra in Fig. 20 exactly at the nodes (i. e. for $k_x = 0$, $k_y = 0$), and slightly away from the nodes (for $k_x = 0.2$, $k_y = 0$).

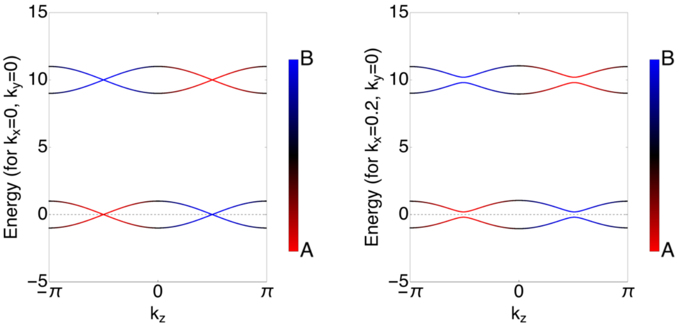


Figure 20: Spectra of the Hamiltonian given in Eq. (S11). The color code shows the orbital content.

In these figures, the color indicates the orbital character, defined by the expectation value of the orbital pseudospin $\langle\tau_z\rangle$. The states at the Weyl nodes are fully orbital polarized, as shown by the following plot of the orbital polarization $\langle\tau_z\rangle$ at $k_x = 0$ and $k_y = 0$ as a function of $k_z$ in Fig. 21.

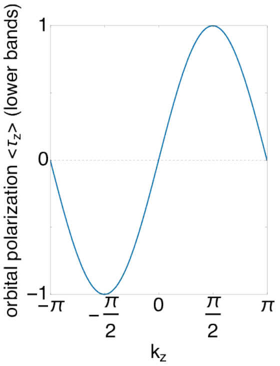


Figure 21: Orbital polarization of the lower two bands of the Hamiltonian given in Eq. (S11).

In the present minimal model, only the states $k_z = \pm k_{\rm Weyl}$ are fully orbital-polarized, and they live in opposite orbitals. This, however, is already enough to decouple the Weyl nodes and avoid any form of interaction-driven gap at the left node: if the interaction is present only in orbital $B$, the electrons exactly at the Weyl node at $k_z = -\pi/2$ are non-interacting (simply because the matrix element of the interaction vanishes for these states). As a result, the electrons at this node are fully decoupled from all other electrons, including the ones at the other Weyl node. This node hence cannot be gapped by the interaction. The momentum range in which the states are orbital-polarized can be increased arbitrarily by the inclusion of longer-range hopping terms.

[1] T. Morimoto and N. Nagaosa, Sci. Rep. **6**, 19853 (2016).
